# Supplementary material for: Bi-CL: A Reinforcement Learning Framework for Robots Coordination Through Bi-level Optimization
Source: arXiv:2404.14649 source file (2024-08-21)
Supplement: Supplementary file 1 [file appendix.tex]

\newpage
\appendix
\section{Experimental Parameters}

\begin{table*}
    \centering
    \caption{Experimental Parameters {\color{blue}Appendix?}}

    \begin{tabular}{cccc}
        \toprule
        \textbf{Parameter} & MAHAC & MADDPG & MAPPO \\ \midrule 
        The number of episode & 5000 & 5000 & 5000 \\ \midrule
        The number of step per episode & 50 & 50 & 50 \\ \midrule
        Discount Factor ($\gamma$) & $0.99$ & $0.99$ & $0.99$ \\ \midrule
        Actor learning rate & $1e-4$ & $1e-4$ & $1e-4$ \\ \midrule
        Critic learning rate & $1e-3$ & $1e-3$ & $1e-3$ \\ \midrule
        Actor network architecture & 256*256*256, ReLU, tanh & 256*256*256, ReLU, tanh & 256*256*256, ReLU, tanh \\ \midrule
        Critic network architecture & 256*256*256, ReLU, linear & 256*256*256, ReLU, linear & 256*256*256, ReLU, linear \\ \midrule
        Batch size & $128$ & $128$ & $128$ \\ \midrule
        Replay buffer size & $1e5$ & $1e5$ & - \\ \midrule
        Target Network Update Frequency & - & $100$ & -  \\ \midrule
        Updates per iteration & - & - & 5 \\ \midrule
        Update batch & $128$ & - & -  \\ \midrule
        Exploration Strategy & $\epsilon$-greedy & Gaussion Noise & -  \\ \midrule
        GAE Lambda & - & - & 0.95  \\ \midrule
        Clip Range & - & - & $0.2$  \\ \bottomrule
    \end{tabular}
    \label{table_training}
\end{table*}
